# Supplementary material for: Uncertainty-Aware Camera Pose Estimation from Points and Lines
Source: arXiv:2107.03890 source file (2021-07-08)
Supplement: Supplementary file 2 [file suppmat.pdf]

# Uncertainty-aware Camera Pose Estimation from Points and Lines (Supplementary Materials)

In this supplementary material we provide additional experimental and theoretical details, namely the covariance propagation which we implemented for the real experiments, further synthetic experiments, and a table illustrating the real experiment. Please also look at the supplementary video for a demonstration of the new methods on the real data.

## 1. Covariance propagation

In real experiments, we triangulate points by minimizing the non-linear least squares reprojection cost taking the 2D detector uncertainty into account:

$$C_p(\mathbf{X}_i) = \left\| \frac{1}{X_i^{(3)}} \begin{bmatrix} X_i^{(1)} \\ X_i^{(2)} \end{bmatrix} - \mathbf{x}_i^l \right\|_{\Sigma_{\mathbf{x}_i^l}}^2 + \quad (1)$$

$$\left\| \frac{1}{X_i^{(3)}} \begin{bmatrix} X_i^{(1)} + b \\ X_i^{(2)} \end{bmatrix} - \mathbf{x}_i^r \right\|_{\Sigma_{\mathbf{x}_i^r}}^2 \rightarrow \min_{\mathbf{X}_i}, \quad (2)$$

where  $b$  is a stereo baseline,  $\mathbf{X}_i = [X_i^{(1)}, X_i^{(2)}, X_i^{(3)}]^T$  is the estimated 3D point,  $\mathbf{x}_i^{\{l,r\}}$  are the point detections for the left and right camera,  $\Sigma_{\mathbf{x}_i^{\{l,r\}}}$  are the corresponding covariance matrices estimated by the point detector. We use a standard covariance propagation approach to estimate the covariance matrix  $\Sigma_{\mathbf{X}_i}$  of  $\mathbf{X}_i$ :

$$\Sigma_{\mathbf{X}_i} = (\mathbf{J}^T \mathbf{J})^{-1} \mathbf{J}^T \text{diag}(\Sigma_{\mathbf{x}_i^l}, \Sigma_{\mathbf{x}_i^r}) \mathbf{J} (\mathbf{J}^T \mathbf{J})^{-1}, \quad (3)$$

where  $\mathbf{J} \in \mathbb{R}^{4 \times 3}$  is a Jacobian corresponding to a non-linear least squares problem (1),  $\text{diag}(\Sigma_{\mathbf{x}_i^l}, \Sigma_{\mathbf{x}_i^r})$  is a block-diagonal  $4 \times 4$  matrix with its  $2 \times 2$  arguments as blocks.

## 2. Synthetic experiments

In this part we provide additional synthetic experiments. We start with justifying specific details of the proposed algorithms, comparing them to the more straightforward baselines. Next we evaluate the performance of the baselines which use only 2D or only 3D uncertainties.

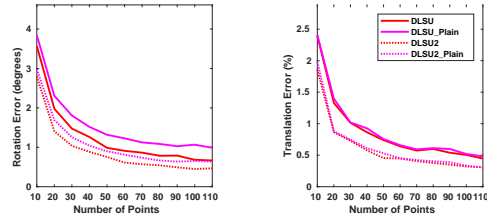

Figure 1. The effect of non-linear refinement on the accuracy of the DLSU and DLSU $\times 2$  methods. DLSU.Plain and DLSU $\times 2$  do not use refinement, while DLSU and DLSU $\times 2$  do. When refinement is used, the accuracy of rotation estimation increases.

## 2.1. Method modifications

### 2.1.1 DLSU Refinement

In this experiment, we justify the improvement in accuracy obtained from the use of the solution refinement stage (end of section 3.1). We perform an experiment with point number variation under 3D uncertainty (Fig. 3, top). We compare a baseline DLSU.Plain and a proposed method DLSU. The results are shown in the Fig. 1. We observe improvement in pose estimation accuracy.

### 2.1.2 EPnPU covariant PCA scheme

Next, we evaluate importance of the algorithm which we propose to construct the matrix  $\mathbf{C}_M$ , described in the beginning of the EPnPU paragraph in section 3.1. We compare the proposed algorithm against a standard PCA-based scheme to construct  $\mathbf{C}_M$ , which we denote as EPnPU.PCA. In the Fig. 2 we see, that the use of the proposed technique results in improvements mainly in translation accuracy.

## 2.2. Separate uncertainties

In the following experiments we compare the methods using full uncertainties with the baselines which use only 2D or only 3D uncertainties. The baselines are obtained by omitting the irrelevant uncertainties in formulas for  $\Sigma_{\mathbf{h}_i}$ ,  $\Sigma_{\mathbf{g}_i}$ . The results are in the Fig. 3. They show that the proposed methods can cope both with 2D and 3D noise while the baselines cannot.

| 2D Points                                                                         | 3D Map                                                                            | EPnP             | EPnPU            | DLSUx2           |
|-----------------------------------------------------------------------------------|-----------------------------------------------------------------------------------|------------------|------------------|------------------|
| 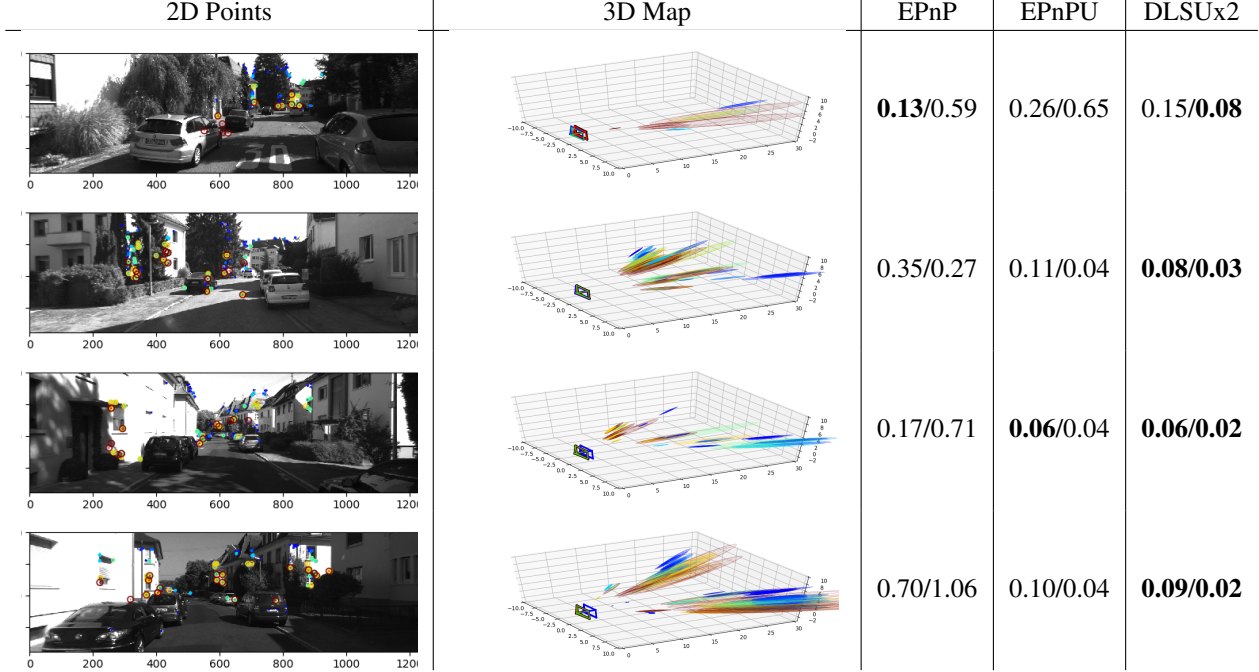 | 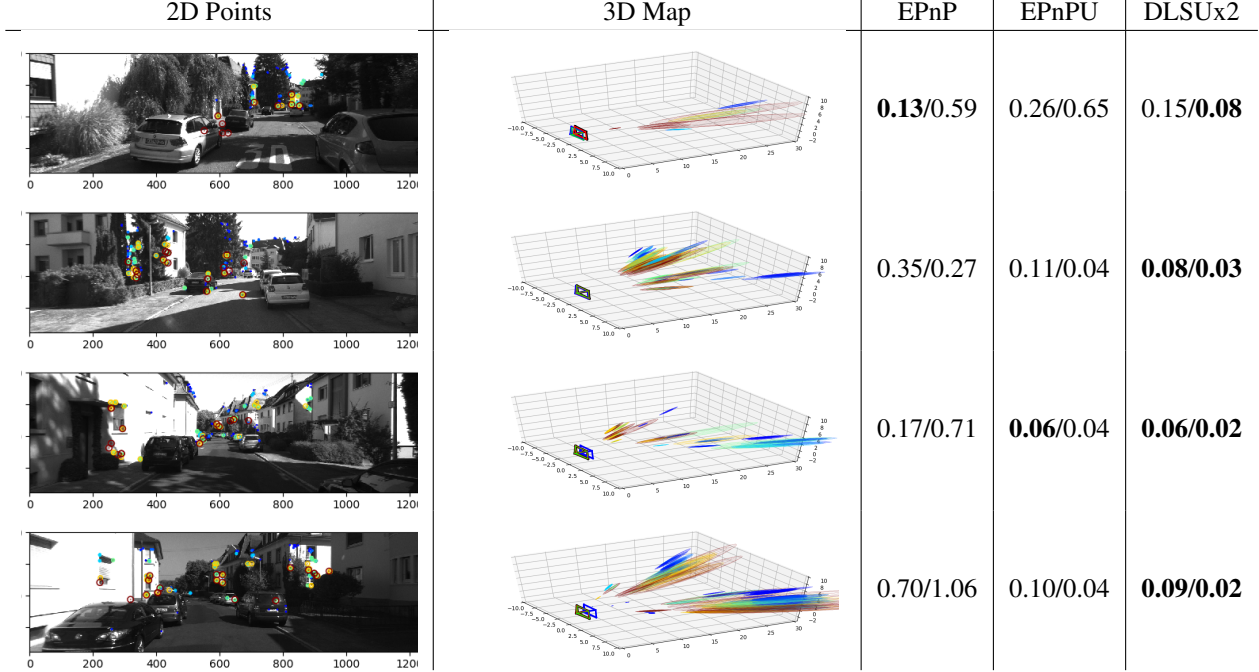 | <b>0.13/0.59</b> | 0.26/0.65        | <b>0.15/0.08</b> |
| 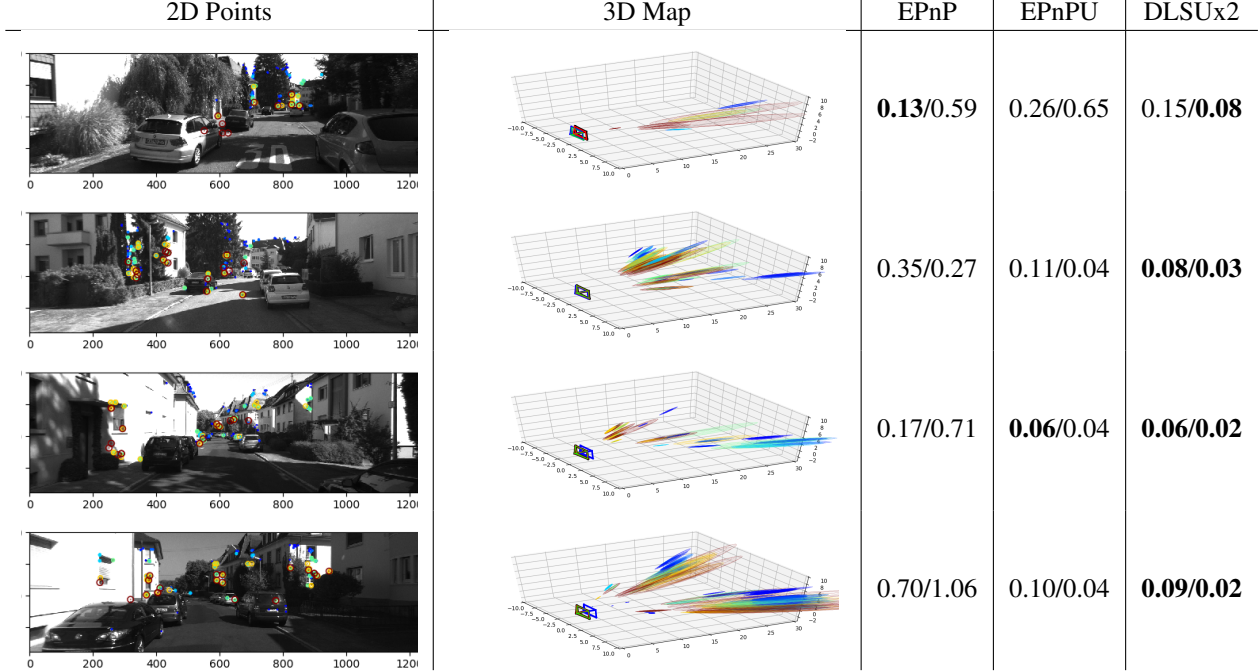 | 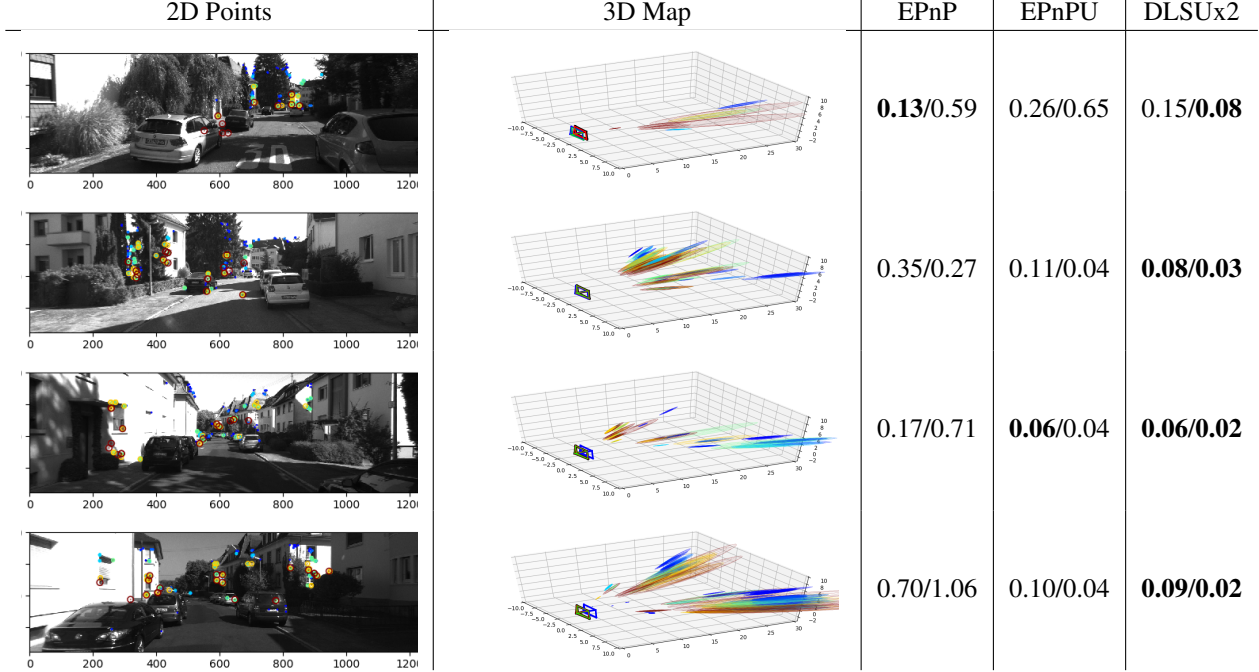 | 0.35/0.27        | 0.11/0.04        | <b>0.08/0.03</b> |
| 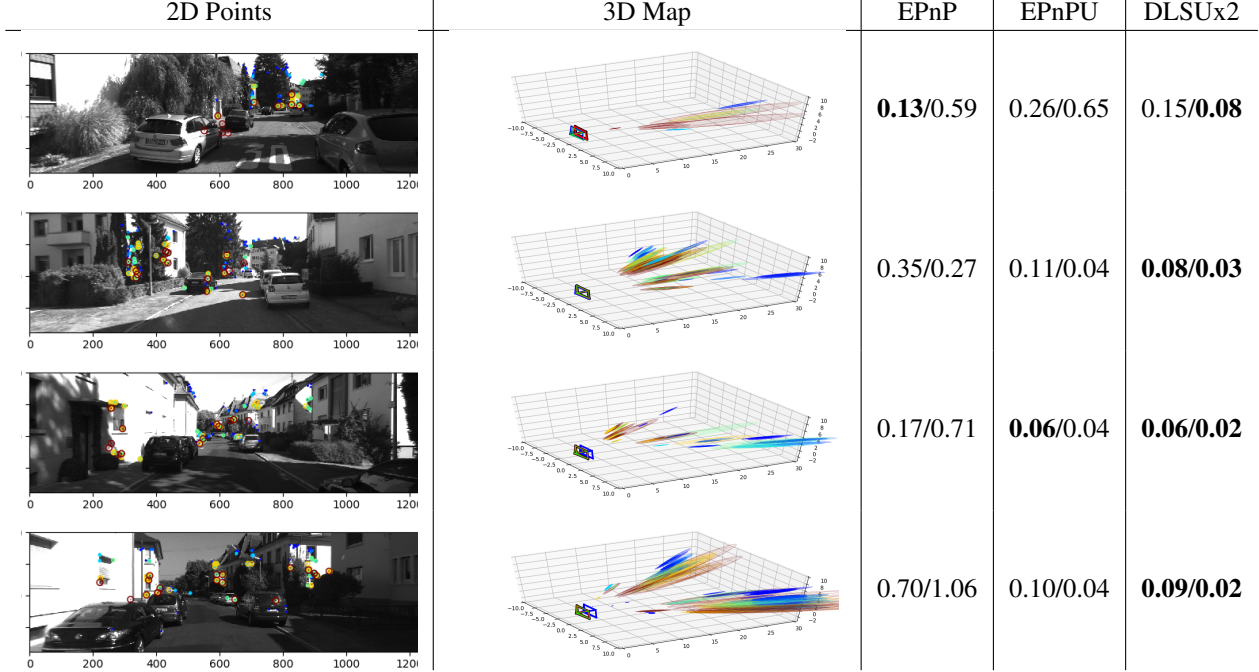 | 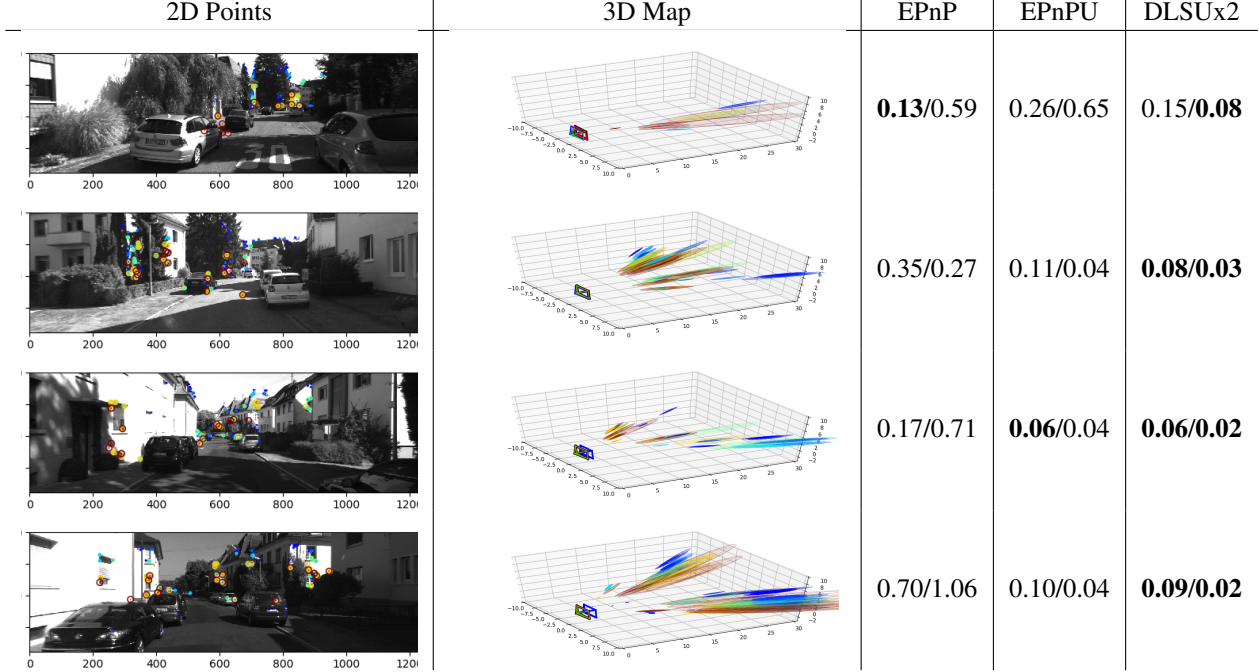 | 0.17/0.71        | <b>0.06/0.04</b> | <b>0.06/0.02</b> |
| 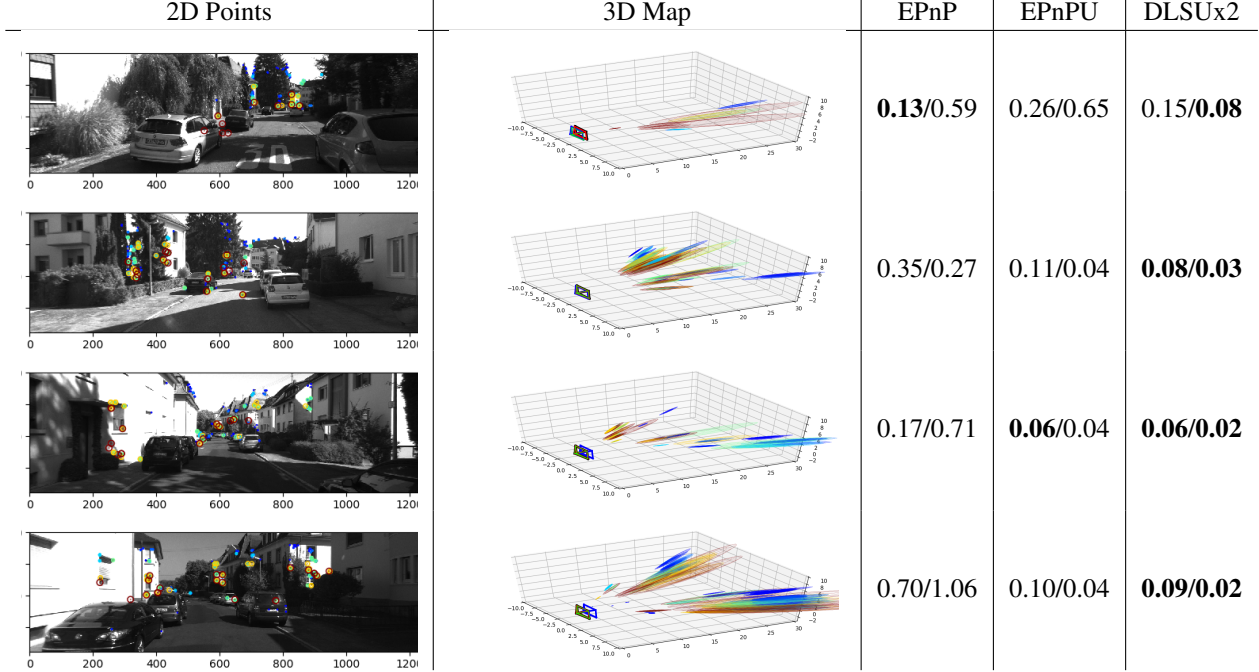 | 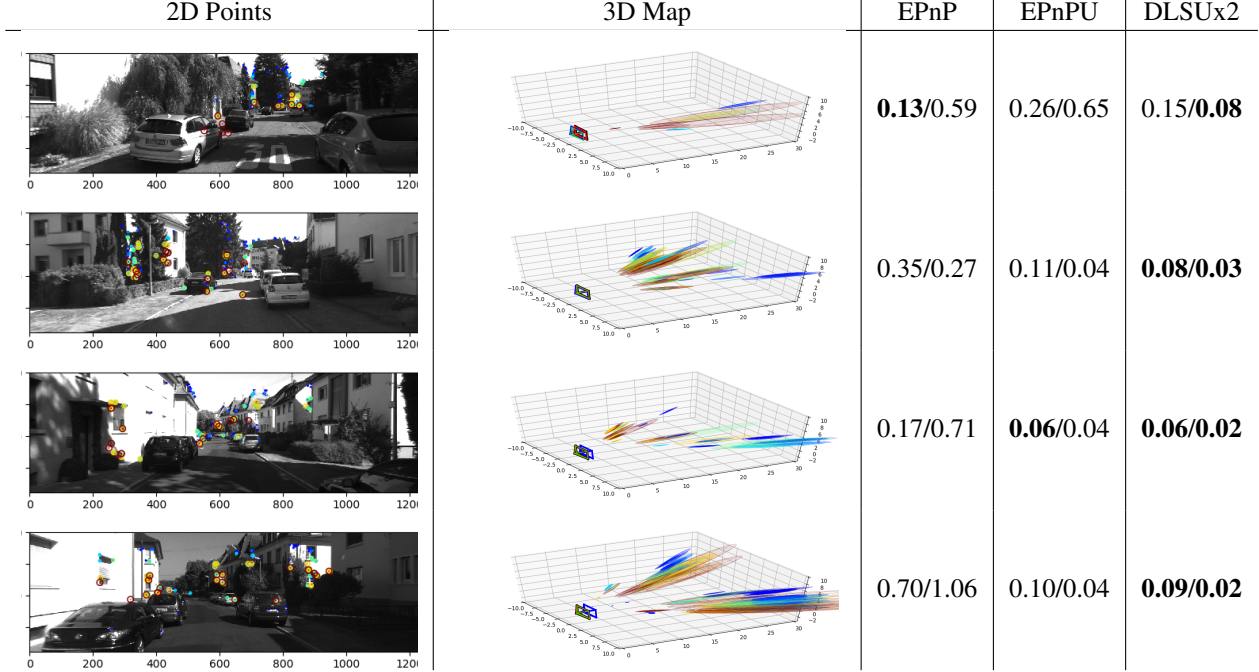 | 0.70/1.06        | 0.10/0.04        | <b>0.09/0.02</b> |

Table 1. The projections of the uncertainties of the DLSUx2 inlier correspondences onto the 2D image, the 3D uncertainties of the same points, and absolute rotation (deg.) and translation (m.) errors for selected frames of the KITTI sequence 00. While in most cases the best performing method DLSUx2 is the most accurate, there are situations when the baseline appears to be more robust (first row). The EPnPU method is sometimes almost as accurate as DLSUx2 (rows 3,4), but in average it has worse translation and rotation accuracy.

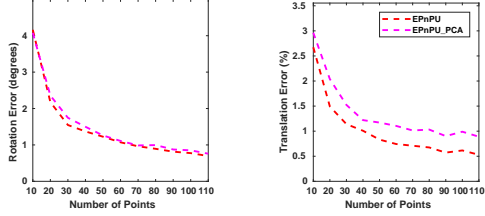

Figure 2. The effect of the proposed algorithm to construct  $C_M$  for the EPnPU method as opposed to the standard PCA-based one. EPnPU\_PCA uses the standard scheme, while EPnPU uses the proposed one. Using the proposed scheme we get higher accuracy of translation estimation.

### 3. Real experiments

In the table 1 we illustrate the real experiments with 2D projections of the uncertainties as well as 3D maps of the uncertainties of the inlier correspondences as estimated by the best-performing DLSUx2 method. We see that although the most accurate in average is DLSUx2, in some cases the baseline EPnP can have better accuracy (first row). The EPnPU method has slightly or significantly worse accuracy than DLSUx2 in these experiments.

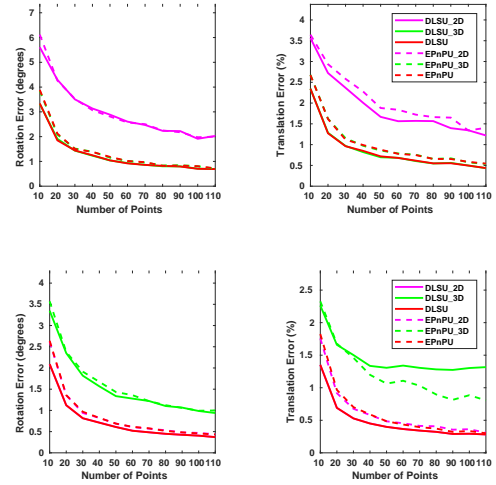

Figure 3. The comparison of the algorithms using 2D, 3D and complete uncertainties. The experiment repeats the 3D (top) or 2D (bottom) noise variation experiment in the main paper (Fig. 3, top or bottom). The median absolute rotation and relative translation errors. The new methods and the 2D-only methods have almost equal accuracy.
